# Supplementary material for: Enhancing HOI Detection with Contextual Cues from Large Vision-Language Models
Source: arXiv:2311.16475 source file (2024-10-08)
Supplement: Supplementary file 1 [file X_suppl.tex]

\clearpage
\setcounter{page}{1}
\maketitlesupplementary
% \balance
\setcounter{section}{0}

% \balance
% \section{Overview}
% In this paper, we introduce three prompts from various perspectives,  utilizing VLM to generate human-centric visual cues within images. To leverage these rich human-centric visual cues, we propose a novel method called HCVC for HOI detection. In this supplementary file, we present a performance comparison between HCVC and InstructBlip in Section B. Additional visualization examples are provided in Section C.
% \label{sec:rationale}
%

\begin{figure*}[t]
\centering
\begin{minipage}{0.89\linewidth}\centering
\centerline{\includegraphics[height=13.0cm]{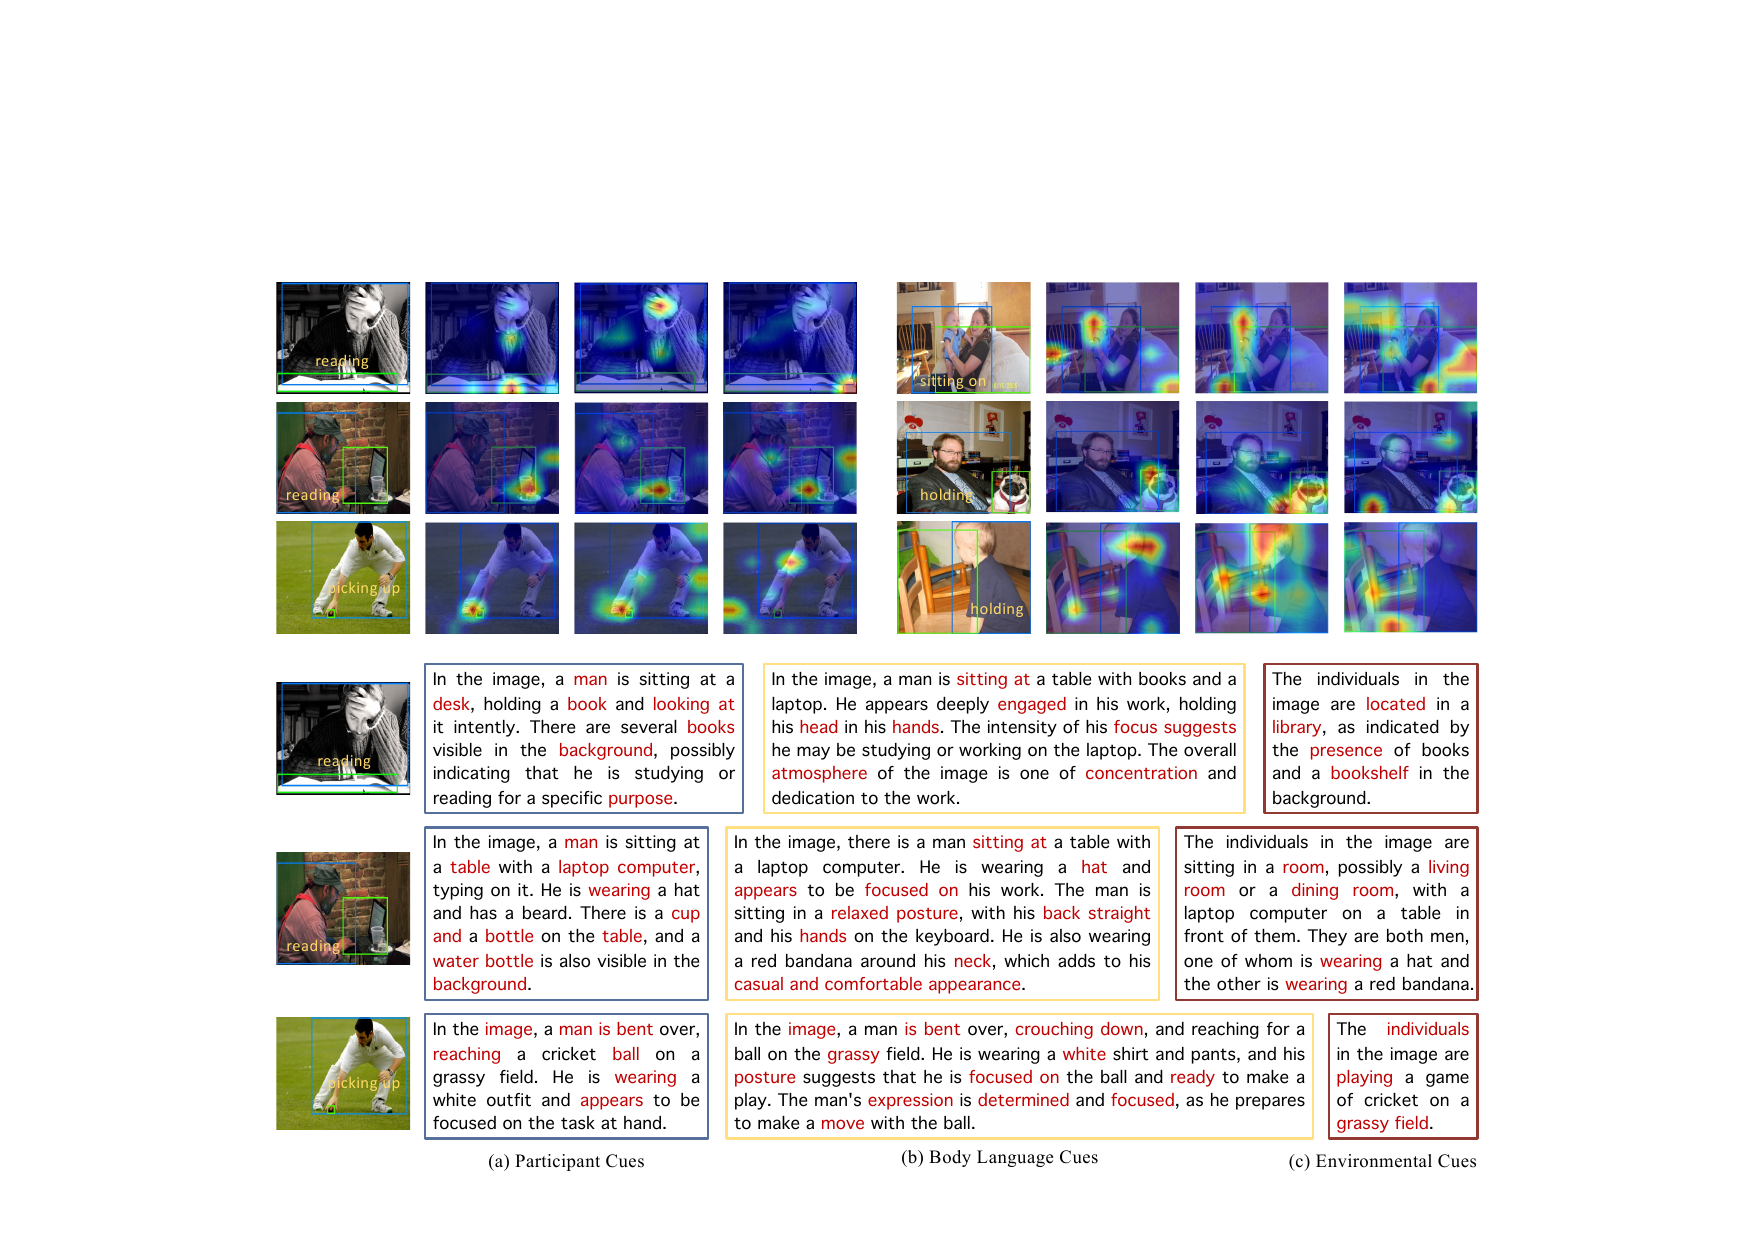}}
\end{minipage}
\vspace{-0.0cm} 
\caption{\textbf{Visualization of predictions.} The upper part is the visualization of spatial feature attention in the interaction decoder, and the lower part is the visualization of visual cue attention in the decoder. The four figures in the upper part from left to right are the prediction results, the spatial attention map about participant cues, body language cues, and environmental cues, respectively. The lower part is marked red if the word's attention exceeds the threshold.}\vspace{-0.0cm} 
\label{visualization_all}\medskip
\end{figure*}

\section{Comparing with InstructBlip}
In this paper, we employ InstructBlip to generate human-centric visual cues in images for Human-Object Interaction (HOI) detection. InstructBlip is a pre-trained model that learns image and text representations on large-scale data. Its notable performance has been demonstrated in various visual information processing tasks. These include image classification and the generation of image captions. 
The effectiveness of InstructBlip lies in its ability to discern and highlight human-centric cues within images, a key aspect of our method.
To thoroughly evaluate the effectiveness of our HCVC, it is crucial to perform a comparative analysis with the InstructBlip method.
\subsection{Task Definition}
Typically, the HOI detection task consists of two subtasks: instance detection and interaction recognition. While existing Vision-Language Models (VLMs) can be utilized to analyze the images by handling interactions between visual content and textual prompts, they are not specifically designed for the traditional HOI detection task. %Especially, these models struggle to effectively focus on detecting objects in the image and providing object localization information.
To compare InstructBlip with our HCVC, we omit the instance detection subtask and primarily focus on interaction recognition. Specifically, given an image $I$, we aim to predict the interaction class between human-object pairs by directly generating the triple tuple $<human, object, interaction>$ from InstructBlip.
\subsection{Prompt for InstructBlip}
To guide InstructBlip in detecting the triple tuple $<human, object, interaction>$ within images, we devise a prompt. The details are as follows:
\begin{center}
\begin{tcolorbox}
[colback=blue!5!white,colframe=blue!45!black,width=0.46\textwidth]
\small
Please analyze the image below and identify the interactions between person(s) and object(s) observed within the image.

$<$Output Format$>$

Each response should be in the format: The person is [interaction label] [object label]

$<$Output Example$>$

The person is playing a sports ball.

The person is holding a laptop.
\end{tcolorbox}
\end{center}

\begin{table}[t]
    \centering \footnotesize
    \begin{tabular}{p{62pt}ccc}
    \toprule
        Method & Full & Rare & Non-Rare \\ \midrule
        InstructBlip & 29.67 & 15.47 & 30.21 \\ 
        \rowcolor{blue!8} HCVC & \textbf{75.52} & \textbf{27.22} & \textbf{77.35} \\ 
        \bottomrule
    \end{tabular}
    \caption{\textbf{Comparisons with InstructBlip under the regular setting on HICO-Det.}}\label{blip1}
\end{table}

% \begin{table}[t]
%     \centering \footnotesize
%     \begin{tabular}{p{57pt}cccc}
%     \toprule
%         Method & Type & Unseen & Seen & Full \\ \midrule
%         InstructBlip & RF-UC & 35.40 & 19.63 & 29.67 \\ 
%         \rowcolor{blue!8} HCVC & RF-UC & \textbf{81.52} & \textbf{58.95} & \textbf{73.32} \\  \hline
%         InstructBlip & NF-UC & \textbf{45.43} & 14.16 & 29.67 \\ 
%         \rowcolor{blue!8} HCVC & NF-UC & 18.01 & \textbf{72.50} & \textbf{45.47} \\ 
%         \bottomrule
%     \end{tabular}
%     \caption{\textbf{Comparisons with InstructBlip under the RF-UC and NF-UC settings on HICO-Det.}}\label{blip2}
% \end{table}

\subsection{Evaluation Metrics}
Most HOI methods employ the following criteria to determine the accuracy of HOI triplet predictions: Firstly, the Intersection over Union (IoU) of the predicted human and object bounding boxes must exceed $0.5$ with respect to the Ground Truth box; secondly, the predicted HOI triplet can exactly match the ground truth. Since we omit the human-object detection sub-task for evaluating the performance of InstructBlip, the first criterion is discarded in our setting. Due to the output limitation of InstructBlip~\footnote{Empirically, InstructBlip often generates one HOI triplet for each image.}, we use top-1 accuracy as the evaluation metric of InstructBlip and our HCVC in this section. In other words, we consider a prediction correct if the first prediction matches the ground truth.
\subsection{Performance Analysis}
The comparison of performance between HCVC and InstructBlip in the regular setting is presented in \cref{blip1}. It can be observed that the performance of HCVC is significantly superior to InstructBlip across the three class sets. Possible reasons for this include: 1) Our HCVC can benefit from both visual and human-centric visual cues features. 2) InstructBlip is a general model and it is not specifically tailored for HOI tasks. %3) InstructBlip may lose some performance during result output as it needs to adhere to specified formats.
From the results, our HCVC outperforms InstructBlip by a large margin, indicating its effectiveness in leveraging visual cues. Additionaly, compared to non-rare categories, InstructBlip's performance drop is less pronounced on rare categories due to its robust generalization capabilities.
% Additionally, we present a performance comparison under zero-shot settings. In most cases, HCVC outperforms InstructBlip significantly in the RF-UC and NF-UC settings. Under the NF-UC setting, where categories with a larger number of data are designated as unseen, HCVC struggles due to a lack of training samples, resulting in poor performance on unseen categories. In contrast, InstructBlip performs well due to its robust generalization capabilities.

In summary, it is clear that the well-designed HCVC approach is significantly better than InstructBlip for the HOI task, demonstrating its effectiveness and superiority.

\section{More Visualization Samples}
In the supplementary materials, we provide additional visualization examples to showcase the performance of HCVC under regular experimental settings, as depicted in \cref{visualization_all}. The upper part presents examples of spatial attention maps within the interaction decoder. The four images from left to right display predicted results, spatial attention maps for participants, body language, and environmental cues, respectively. HCVC yields accurate predictions, and the interaction decoder, using different cues, focuses on different regions. This highlights the necessity of not sharing parameters among the three decoders.

Furthermore, we conducted an attention analysis of words in each cue for three of the images. Words exceeding the threshold are highlighted in red. From these highlighted words, we can more easily understand the basis of the model's judgments, enhancing interpretability. For instance, in the first image, HCVC extracts information from participant cues that there is a man, a book, and a table in the image. Although there are some inaccuracies in the body language cues generated by VLM, such as ``the presence of a computer'', HCVC focuses on the fact that the man is seated and engaged in his work. From environmental cues, HCVC deduces that this is in a library with a bookshelf. Finally, HCVC collects information from these cues and integrates them with visual features to infer that the interaction type is ``a person \textcolor{red}{reading} a book''.
% \balance
